# Supplementary material for: Grid-based minimization at scale: Feldman-Cousins corrections for SBN
Source: arXiv:2002.07858 source file (2020-02-18)
Supplement: Supplementary file 1 [file appendix.tex]

This is my appendix.  Hope it does not burst.

\bigskip
\noindent
Function list:

\begin{description}[style=unboxed,leftmargin=0cm]
\item $Smear: (GenState, Spectrum) \rightarrow (GetState, Spectrum)$
\item $Signal: Point \rightarrow Spectum$
\item $CalcX^2: (Spectrum, Spectrum) \rightarrow \mathbb{R}$
\item $FindMinSig: (f:Point \rightarrow double, Grid) \rightarrow (Point, Spectrum)$
\item $Make\Delta X^2: (GenState, Spectrum, Spectrum, Grid) \rightarrow (GenState, \mathbb{R})$
\item $Make\Delta X^2Hist: (Point, Spectrum, Grid) \rightarrow Hist$
\item $FindCriticalValue: (GenState, Point, Spectrum, Grid) \rightarrow \mathbb{R}$
\end{description}

% $f \circ g$

\bigskip
\noindent
Algorithm:

\begin{description}
\item $CalcX^2(a, b): \\
  \text{calculate chi2 from the spectrums a and b}$
\item $Make\Delta X^2(st, sp, c, G): \\
  smeared, st = smear(st, sp) \\
  q_{min}, q_{sig} = FindMinSig (CalcX^2(smeared) \circ signal, G)  \\
  CalcX^2(sp, c) - CalcX^2(sp, q_{sig})$
\item $Make\Delta X^2Hist(p, c, G): \\
  take(1000, Make\Delta X^2(signal(p), c, G)$
\item $FindCriticalValue(p, c, G): \\
  h=Make\Delta X^2Hist(p, c, G) \\
  \text{do work to find the delta chi2 value from h}$ 
\item $Result = Map( FindCriticalValue(c, G), G)$
\end{description}

\bigskip
Note:
 c = C(p) for p in G ? i.e. it depends on point p

Finding q such that chi2 is minimum using all of G (inner loop)
I think this use of the full grid is an implementation choice and actually is a red herring for us.  
The most interesting region for this part of the calculation is  likely to extend out in the neighborhood of p where sp=signal(p).
I do not think the q that minimizes chi2 value will not be found far from p (far meaning most of G that is distant from p)
The points that are explored for finding minimum chi2 q should just be built up in the running of this portion of the algorithm

The grid G use overall in the application
I think it is also uninteresting to predetermine this entire space as a regular grid
G could be any set of points or a collection of interesting regions, or whatever. 
Main idea is to exclude any place that is not going to yield interesting values.  With the concept of the entire grid gone in finding q with chi2 minimum, it is likely going to be feasible to explore using the actual statistic at an arbitrary point in parameter space.
